# Supplementary material for: Predicting the Charge Density Response in Metal Electrodes
Source: arXiv:2304.08966 ancillary file (2023-08-20)
Supplement: Supplementary file 1 [file supplemental_material.pdf]

# Predicting the Charge Density Response in Metal Electrodes - Supplemental Material

Andrea Grisafi,[1,*] Augustin Bussy,[2] Mathieu Salanne,[3,4] and Rodolphe Vuilleumier[1]

[1] *PASTEUR, Département de chimie, École Normale Supérieure, PSL University, Sorbonne Université, CNRS, 75005 Paris, France*
[2] *Department of Chemistry, University of Zurich, Winterthurerstrasse 190, 8057 Zürich, Switzerland*
[3] *Sorbonne Université, CNRS, Physicochimie des Électrolytes et Nanosystèmes Interfaciaux, F-75005 Paris, France*
[4] *Institut Universitaire de France (IUF), 75231 Paris, France*

## DATASETS GENERATION

Training configurations associated with the gold electrodes of increasing size are generated by considering symmetric Au(100) slabs made of 2 unit cell repetitions along the $xy$ plane and spanning from $n_{\mathrm{L}}$=3 to $n_{\mathrm{L}}$=15 atomic layers along $z$. In particular, we consider uniform random displacements of the atomic positions up to 2.5% of the lattice constant along the three Cartesian directions and build a total of 240 electrode configurations made of 40 structures for each slab size from $n_{\mathrm{L}}$=3 to $n_{\mathrm{L}}$=11, 20 structures for $n_{\mathrm{L}}$=13 and 20 structures for $n_{\mathrm{L}}$=15.

The ionic capacitor considered in this work was defined from a rigid Au(100) electrode made of 4 unit cell repetitions along the $xy$ plane and 7 metal layers along $z$, which is put in contact with a concentrated water/NaCl solution under a uniform electric field $E_z = 0.016$ V/Å. In particular, we consider 200 water molecules and 20 NaCl ion pairs, that, together with the gold electrode, occupy a box size of $L_{x/y} = 11.54$Å and $L_z = 64.34$Å. In line with Ref. [1], this choice is such to allow for the simulation of an ionic capacitor subject to an applied voltage $\Delta V = -E_z \times L_z = -1.0$V. Finite-$E$ classical reference trajectories were then obtained thanks to the MetalWalls program [2], which includes a specific implementation suitable to simulate the polarization of the metal electrode along $z$ through the fluctuation of opposite atomic Gaussian charges at the two metal surfaces [1]. In particular, training configurations were generated by selecting 2000 uncorrelated frames in times steps of 2 ps from a finite-$E$ trajectory of 10 ns, run using a Nosé–Hoover thermostat [3] at $T$=298K and a TIP4P/2005 model of water [4]. 5500 test configurations were similarly selected from an another trajectory of 30 ns run with the same thermodynamic conditions in order to provide an estimate of the differential capacitance of the system.

For all the examples considered, reference electron densities $n_e$ are computed at the DFT/PBE level using the open source CP2K simulation package [5] with ccGRB-D basis sets (distributed as part of the CP2K package from version 9.1) and GTH pseudo-potentials [6]. In the case of gold slabs of increasing size, we further set a vacuum space of twice the metal thickness on both sides of the slab and adopt a Martyna-Tuckerman correction suitable to screen the electrostatic potential along the non-periodic $z$-direction [7, 8]. Both for the case of Au(100)/$Na^+$ and Au(100)/electrolyte, we rely on the QM/MM implementation reported in Ref. [9]. External fields are applied by evaluating an external potential of the form $\phi^{\text{ext}} = -E_z z$ over the CP2K real-space grids. In the case of the 3D-periodic Au(100)/electrolyte example, the gold electrode has been set in the center of the simulation box in order to have the discontinuous jump of the external potential in the classical electrolyte region. MM charges are set consistently with the classical MetalWalls simulation as $q_{\mathrm{Na}} = +1.0|e|$, $q_{\mathrm{Cl}} = -1.0|e|$, $q_{\mathrm{M}} = -1.1128|e|$ and $q_{\mathrm{H}} = +0.5564|e|$.

### Density-fitting approximation

In order to have the electron density in a form suitable for learning, we recast the Kohn-Sham electron density over a linear basis. In particular, we consider the linear expansion of the electron density on an atom-centered auxiliary basis $\tilde{\chi}_k$ given by the product of radial functions $R_n^\lambda$ and spherical harmonics $Y_{\lambda\mu}$, so that $k = (n\lambda\mu)$ represents a compact basis function index. In order to take into account the two dimensional periodicity of the system on the $xy$-plane, we shall consider the sum of the basis functions over 2D-periodic images:

$$n_e^{\mathrm{DF}}(\mathbf{r}) = \sum_{ik} \sum_{ix,iy} c_i^k \tilde{\chi}_k(\mathbf{r} - \boldsymbol{r}_i - \boldsymbol{u}_{ix,iy}) \,, \tag{S1}$$

where $\boldsymbol{r}_i$ are the atomic positions in the unit cell and $\boldsymbol{u}_{ix,iy} = (u_x, u_y, 0)$ is the cell translation vector.

To compute the expansion coefficients $c_k^i$, we adopt a global density-fitting (DF) strategy using an overlap metric. Therefore, we minimize the integrated square error between the self-consistent Khon-Sham electron density and its DF approximation:

$$\arg\min_{\boldsymbol{c}} \int d\mathbf{r} \left(n_e^{\mathrm{DF}}(\mathbf{r}) - n_e^{\mathrm{KS}}(\mathbf{r})\right)^2 \,, \tag{S2}$$

which gives the DF expansion coefficients as

$$\boldsymbol{c} = \boldsymbol{S}^{-1}\boldsymbol{w} \,. \tag{S3}$$

The matrix $\boldsymbol{S}$ contains the 2-center overlap integral between auxiliary functions, $S_{kk'} = \langle \tilde{\chi}_{k'} | \tilde{\chi}_k \rangle$, while the vector $\boldsymbol{w}$ contains the projections of the Kohn-Sham density on the auxiliary functions $w_k = \left\langle \tilde{\chi}_k \middle| \Delta n_e^{\mathrm{KS}} \right\rangle$. In this work, all density fitting calculations use the RI-HFX implementation of CP2K [10], where all integrals and contractions are

taken care of internally. The DF expansion coefficients $\boldsymbol{c}$ of equation (S3) are a direct output of such calculation. Note that despite using Hartree–Fock machinery, the pure PBE density is fitted (calculations with 0% of HF exchange, and the overlap RI metric/HF potential). The auxiliary DF basis set used in this work is a fully uncontracted version of the automatically generated basis set obtained using the method of Stoychev and co-workers [11]. The basis set amounts to 224 functions per gold atom, with up to $\lambda = 6$ spherical harmonics.

## LONG-DISTANCE EQUIVARIANTS

We summarize here the derivation the $\rho \times V$ long-distance equivariant (LODE) representation as reported in Ref. 12. We start by considering a smooth atom-density representation of a local environment of the atom $i$:

$$\rho_i^a(\mathbf{r}) = f_{\text{cut}}(r) \sum_{j\in a} e^{-\alpha|\boldsymbol{r}-\boldsymbol{r}_{ij}|^2} \,, \tag{S4}$$

with $j$ running over the atomic neighbours of the atom $i$ which belong to a given atomic species $a$, $\alpha$ is the Gaussian decay factor and $f_{\text{cut}}$ is a cutoff function of radius $r_{\text{cut}}$. Similarly, we define a smooth Coulomb-like potential representation of a local environment of the atom $i$:

$$V_i^a(\mathbf{r}) = f_{\text{cut}}(r) \int_\Omega d\boldsymbol{r}' \frac{\sum_{j\in a} e^{-\alpha|\boldsymbol{r}'-\boldsymbol{r}_{ij}|^2}}{|\boldsymbol{r}-\boldsymbol{r}'|} \,. \tag{S5}$$

We now consider the symmetry adapted tensor product of $\rho_i^a$ and $V_i^a$ so that to reflect the rotational symmetry of spherical tensors of order $\lambda$. In a compact abstract notation, this can be written in terms of the following rotational average [13]:

$$\int d\hat{R} \left( \hat{R} \left|\rho_i^a\right\rangle \otimes \hat{R} \left|V_i^{a'}\right\rangle \otimes \hat{R} \left|\lambda\mu\right\rangle \right) \tag{S6}$$

with $\hat{R}$ the rotation operator. Upon expanding $\rho_i^a$ and $V_i^a$ in spherical harmonics ($|lm\rangle$ and $|l'm'\rangle$) and discretizing the radial coordinates with a set of orthogonal radial functions ($|n\rangle$ and $|n'\rangle$), the rotational average of Eq. (S6) yields a structural descriptor $P_i^{\lambda\mu}$ which is equivariant in $SO(3)$:

$$P_i^{\lambda\mu}(aa'nn'll') = \sum_{mm'} \rho_i^{anlm} \, V_i^{a'n'l'm'} \left\langle lm, l'm' | \lambda\mu \right\rangle \,, \tag{S7}$$

where $\langle lm; l'm' | \lambda\mu\rangle$ are Clebsch–Gordan coefficients and the combination of indexes $(aa'nn'll')$ identifies the feature space of $P_i^{\lambda\mu}$. Retaining only the components for which $l + l' + \lambda$ is even is then enough to further enforce equivariance in $O(3)$, including inversion operations [14].

## FINITE-FIELD EXTENSION OF LODE

We report here a detailed derivation of the finite-field extension of the LODE method introduced in the main text. We shall consider in particular the application of a constant and uniform electric field along $z$, $E_z$. To include this information within the structural descriptor, we add a term of the form $E_z\, z$ which replaces the definition of the potential of Eq. (S5), i.e.,

$$V_i^E(\boldsymbol{r}) = E_z\,(z - z_i)\, f_{\text{cut}}(r) \tag{S8}$$

Note that as the potential reference does not bring any information to the effect of the external field on the local environment, we set the potential origin at the position of the central atom $i$, i.e., $V_i^E(\boldsymbol{r}_i) \equiv 0$. From this definition, the spherical harmonic components of $V^E$ about any given atom $i$ read as follows,

$$V_i^{nlm,E} = \sqrt{\frac{4\pi}{3}} E_z \left( \int_0^\infty dr\, r^3 R_n(r) \right) \delta_{l1}\delta_{m0} \,. \tag{S9}$$

where $R_n(r)$ are orthogonal radial functions analogous to those used to expand the Gaussian density and Coulomb potential fields [15, 16]. Plugging Eq. (S9) into Eq. (S7), the resulting descriptor equivariant in $SO(3)$ is

$$P_i^{\lambda\mu,E}(ann'll') = \sqrt{\frac{4\pi}{3}} E_z \left( \int_0^\infty dr\, r^3 R_{n'}(r) \right) \sum_m \rho_i^{anlm} \langle lm; 10 | \lambda\mu \rangle \; . \tag{S10}$$

Note that from the rules of angular momentum composition, $\mu = m + 0$ and $|l - 1| \leq \lambda \leq (l + 1)$ in the previous equation. Thus, the possible values for $l$ are restricted to $(\lambda + 1, \lambda, |\lambda - 1|)$, while $m = \mu$. Moreover, enforcing the covariance under inversion operations implies $l + 1 + \lambda$ must be even, so that only the two values $l = |\lambda \pm 1|$ survive. The final finite-field extension of the LODE descriptor is obtained as the direct sum of $P_i^{\lambda\mu}$ and $P_i^{\lambda\mu,E}$, which upon normalization of the individual input vectors, can be conveniently implemented in kernel space by taking the simple sum of the corresponding kernels:

$$\tilde{\boldsymbol{k}}_{ij}^{\lambda,E} = \boldsymbol{k}_{ij}^{\lambda} + \boldsymbol{k}_{ij}^{\lambda,E} \; . \tag{S11}$$

Note that particular care must be taken when making the model non-linear. In fact, given that the field $E_z$ is rigidly attached to the frame of reference of the simulation box, $P_i^{00,E}$ is not invariant under a rigid rotation of the system, but it will transform following the symmetry of ($l = 1$; $m = 0$) spherical harmonics. Therefore, a non-linear equivariant kernel that preserves the field symmetry can be constructed as follows:

$$\tilde{\boldsymbol{k}}_{ij}^{\lambda,E} = \left( \boldsymbol{k}_{ij}^{\lambda} + \boldsymbol{k}_{ij}^{\lambda,E} \right) \times k_{ij}^{0} \; , \tag{S12}$$

where $k_{ij}^0$ is the rotationally invariant ($\lambda = 0$) LODE kernel. Note that this multiplication also allows us to introduce an effective coupling between the LODE structural features and the external field, which are instead disregarded in the linear model of Eq. (S11).

## MACHINE-LEARNING PARAMETERS

We report here details about the hyperparameters used within the Symmetry-Adapted Learning of Three-Dimensional Electron Densities (SALTED) method, which follows the implementation reported in Ref. [17]. As already described in the main text, within SALTED an equivariant kernel-based approximation of the density expansion coefficients is provided as $\boldsymbol{c}_i^{n\lambda} = \sum_M \boldsymbol{k}_{iM}^{\lambda} \boldsymbol{b}_M^{n\lambda}$. A crucial aspect is the selection of a sparse set $\{M\}$ of atomic environments that are representative of the structural variations of the training set. Together with the size of the basis set used for the expansion of the electron density, this parameter defines the final dimensionality of the regression problem [17]. In this work, the selection of atomic environments is performed using the farthest-point sampling (FPS) method [18] based on SOAP and LODE metrics, depending on the specific model at hand. In particular, we used $M = 200$ for the Au(100)/$Na^+$ example, $M = 150$ for the Au(100) electrodes under an external field, and $M = 800$ for the Au(100)/electrolyte example. To avoid overfitting, a regularization parameter $\eta = 10^{-8}$ is used for the electrodes of increasing size, while a value of $\eta = 10^{-20}$ has been used for the Au(100)/electrolyte example.

Given the chosen basis set for the electron-density expansion, equivariant descriptors vectors $\boldsymbol{P}_i^{\lambda}$ for each atom $i$ included in the training set are computed up to $\lambda = 6$ in order to mirror the $O(3)$ symmetry of the atom-centered density components. From these descriptors, symmetry-adapted sparse kernel functions $\boldsymbol{k}_{iM}^{\lambda}$ are then obtained from the inner product between pairs of $\boldsymbol{P}_i^{\lambda}$ [19]. To improve the learning performance without affecting the problem dimensionality, non-linear kernels are then computed by multiplying each symmetry-adapted kernel of order $\lambda$ by its scalar $\lambda = 0$ counterpart [20], i.e., $\boldsymbol{k}_{ij}^{\lambda} \times \left(k_{ij}^{0}\right)^{\zeta - 1}$, with $\zeta$ a positive integer chosen to modulate the degree of non-linearity. In this work, we used $\zeta = 2$ for the electrodes of increasing size and $\zeta = 1$ for the ionic capacitor example.

The calculation of atom density and potential spherical harmonics projections, $\rho_i^{anlm}$ and $V_i^{anlm}$, entering the calculation of the equivariant descriptors $\boldsymbol{P}_i^{\lambda}$ was performed using the rascaline package [21]. For both the first two examples including electrodes of increasing size, we construct atom density and potential fields using Gaussian widths of $\sigma = 0.5$ Å and $\sigma = 4.0$ Å with a cutoff of $r_{\text{cut}} = 8$ Å. $\rho$-fields are discretized using up to $l_{\text{cut}} = 6$ spherical harmonics and $n_{\text{cut}} = 6$ radial functions, while we adopted $l_{\text{cut}} = 3$ and $l_{\text{cut}} = 3$ for the $V$-fields. As for the ionic capacitor example, atom density and potential fields were constructed using Gaussian widths of $\sigma = 0.5$ Å and $\sigma = 1.0$ Å with a cutoff of $r_{\text{cut}} = 10$ Å. Each field was then discretized with $l_{\text{cut}} = 6$ and $n_{\text{cut}} = 6$.

## CHARGE CONSERVATION

A crucial aspect of the method for the calculation of derived electrostatic properties consists in guaranteeing that the predicted electron density response $\Delta n_e$ integrates to 0. In this work, this condition is enforced exactly by *a posteriori* subtraction of the excess electronic charge $\Delta q_e$ from the isotropic ($\lambda$=0, $\mu$=0) density coefficients associated with the most diffuse radial functions $R^0_{n_{\max}}$:

$$\tilde{c}_i^{n_{\max}00} = c_i^{n_{\max}00} - \frac{1}{N_{\rm at}} \frac{\Delta q_e}{\sqrt{4\pi}\int_0^\infty dr\, r^2\, R^0_{n_{\max}}(r)}\,, \tag{S13}$$

with the excess electronic charge given by

$$\Delta q_e = \int_\Omega d\mathbf{r}\, \Delta n_e^{\rm ML}(\mathbf{r}) = \sqrt{4\pi}\sum_i\sum_n c_i^{n00}\int_0^\infty dr\, r^2\, R^0_n(r)\,. \tag{S14}$$

We report below Tables that include the predicted excess electronic charge $\Delta q_e$ associated with the test electrode of increasing size $n_{\rm L}$ considered in this work. For LODE models, we observe small absolute charge conservation errors $|\Delta q_e| < 0.01e$. Conversely, SOAP is associated with large errors $|\Delta q_e| > 0.1e$, remarking the inadequacy of a local model to extrapolate the long-range response of the metal electrodes.

| $n_{\rm L}$ | 19 | 21 | 23 | 25 | 27 |
|---|---|---|---|---|---|
| SALTED/SOAP | -0.1360 | -0.1645 | -0.1931 | -0.2216 | -0.2502 |
| SALTED/LODE | 0.0078 | 0.0082 | 0.0076 | 0.0061 | 0.0037 |

TABLE S1. Excess electronic charge $\Delta q_e$, in atomic units, associated with the prediction of $\Delta n_e$ for the test Au(100) electrodes interacting with a classical $Na^+$ ion considered in this work.

| $n_{\rm L}$ | 19 | 21 | 23 | 25 | 27 |
|---|---|---|---|---|---|
| SALTED/LODE+E | -0.0024 | -0.0003 | 0.0059 | -0.0008 | -0.0014 |

TABLE S2. Excess electronic charge $\Delta q_e$, in atomic units, associated with the prediction of $\Delta n_e$ for the test Au(100) electrodes under an applied electric field considered in this work.

## CALCULATION OF THE ELECTRONIC POLARIZATION

From the predicted electron density response $\Delta n_e$, the polarization along the non-conducting direction $z$ is given by

$$p_z = -\int_\Omega d\mathbf{r}\, z\, \Delta n_e(\mathbf{r})\,. \tag{S15}$$

This can be readily computed from the ($\lambda$=0, $\mu$=0) and ($\lambda$=1, $\mu$=0) electron density coefficients:

$$\begin{aligned}
\int_\Omega d\mathbf{r}\, z\, \Delta n_e(\mathbf{r}) &= \int_\Omega d\mathbf{r}\, z\left[\sum_i\sum_{n\lambda\mu} c_i^{n\lambda\mu}\sum_{ix,iy} R^\lambda_n(|\mathbf{r}-\mathbf{r}_i-\boldsymbol{u}_{ix,iy}|)Y_{\lambda\mu}(\widehat{\mathbf{r}-\mathbf{r}_i-\boldsymbol{u}_{ix,iy}})\right]\\
&= \sum_i\sum_{n\lambda\mu} c_i^{n\lambda\mu}\int_\Omega d\mathbf{r}\,(z-z_i+z_i)\sum_{ix,iy} R^\lambda_n(|\mathbf{r}-\mathbf{r}_i-\boldsymbol{u}_{ix,iy}|)Y_{\lambda\mu}(\widehat{\mathbf{r}-\mathbf{r}_i-\boldsymbol{u}_{ix,iy}})\\
&= \sum_i\sum_{n\lambda\mu} c_i^{n\lambda\mu}\left[z_i\sqrt{4\pi}\delta_{\lambda0}\delta_{\mu0}\int_0^\infty dr\, r^2 R^\lambda_n(r) + \sqrt{\frac{4\pi}{3}}\delta_{\lambda1}\delta_{\mu0}\int_0^\infty dr\, r^3 R^\lambda_n(r)\right]\\
&= \sum_i\sum_n\left[c_i^{n00}\, z_i\sqrt{4\pi}\int_0^\infty dr\, r^2 R^0_n(r) + c_i^{n10}\sqrt{\frac{4\pi}{3}}\int_0^\infty dr\, r^3 R^1_n(r)\right]\,,
\end{aligned} \tag{S16}$$

where the radial integrals are all analytically computed.

## COMPUTATIONAL EFFICIENCY

We report below an analysis of the computational efficiency associated with the prediction of the Au(100)/$Na^+$ charge density response over electrodes of increasing size, comparing the CPU time of the reference DFT calculations with that of SALTED/SOAP and SALTED/LODE predictions. We observe that both ML models present a speedup of the order of $10^3$ with respect to DFT, which progressively increases with the electrode size. We note that because of the smooth Gaussian density used for the construction of the LODE potential, the performance and asymptotic scaling of SALTED/LODE is similar to that of SALTED/SOAP. In this context, the slight speedup of LODE with respect to SOAP is due to the reduced feature space of the former model, deriving from having used a smaller number of angular and radial functions to expand the atomic potential $V_i$ with respect to the expansion of the atomic density $\rho_i$.

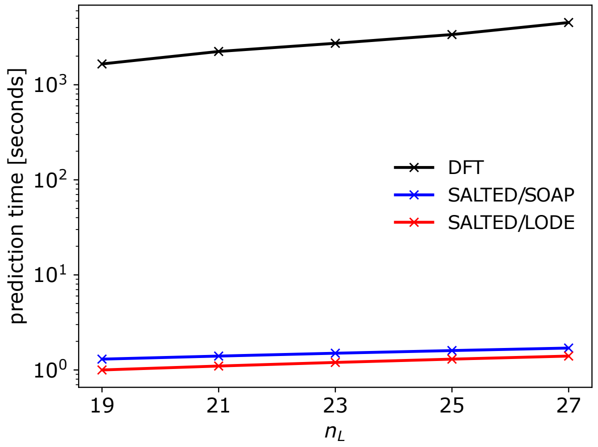


FIG. S1. Prediction time as a function of the number of metal layers $n_{\mathrm{L}}$ associated with the Au(100)/$Na^+$ charge density response obtained from SALTED/SOAP (blue line) and SALTED/LODE (red line) calculations parallelized on 24 CPUs, as compared with the reference DFT time (black line).

## CALCULATION OF THE HARTREE POTENTIAL

From the predicted electron density response $\Delta n_e$, the response of the Hartree potential is defined as follows:

$$\Delta\phi_{\mathrm{H}}(\mathbf{r}) = -\int d\mathbf{r}' \, \frac{\Delta n_e(\mathbf{r}')}{|\mathbf{r}' - \mathbf{r}|} \, . \tag{S17}$$

In practice, the calculation of $\Delta\phi_{\mathrm{H}}$ is performed by feeding the predicted density coefficients back into the CP2K code [5], already used to perform the reference DFT calculations. We report in Fig. S2 the extrapolation results for the Hartree potential drop induced by the interaction of the test Au(100) electrodes with a sodium cation (represented as a classical Gaussian charge) placed at 4Å distance from the upper metal surface. SOAP models come along with a predicted Hartree potential drop that is progressively less accurate upon increasing the number of metal layers $n_{\mathrm{L}}$. Conversely, LODE-based predictions yield an excellent agreement of the potential drop at all electrode sizes.

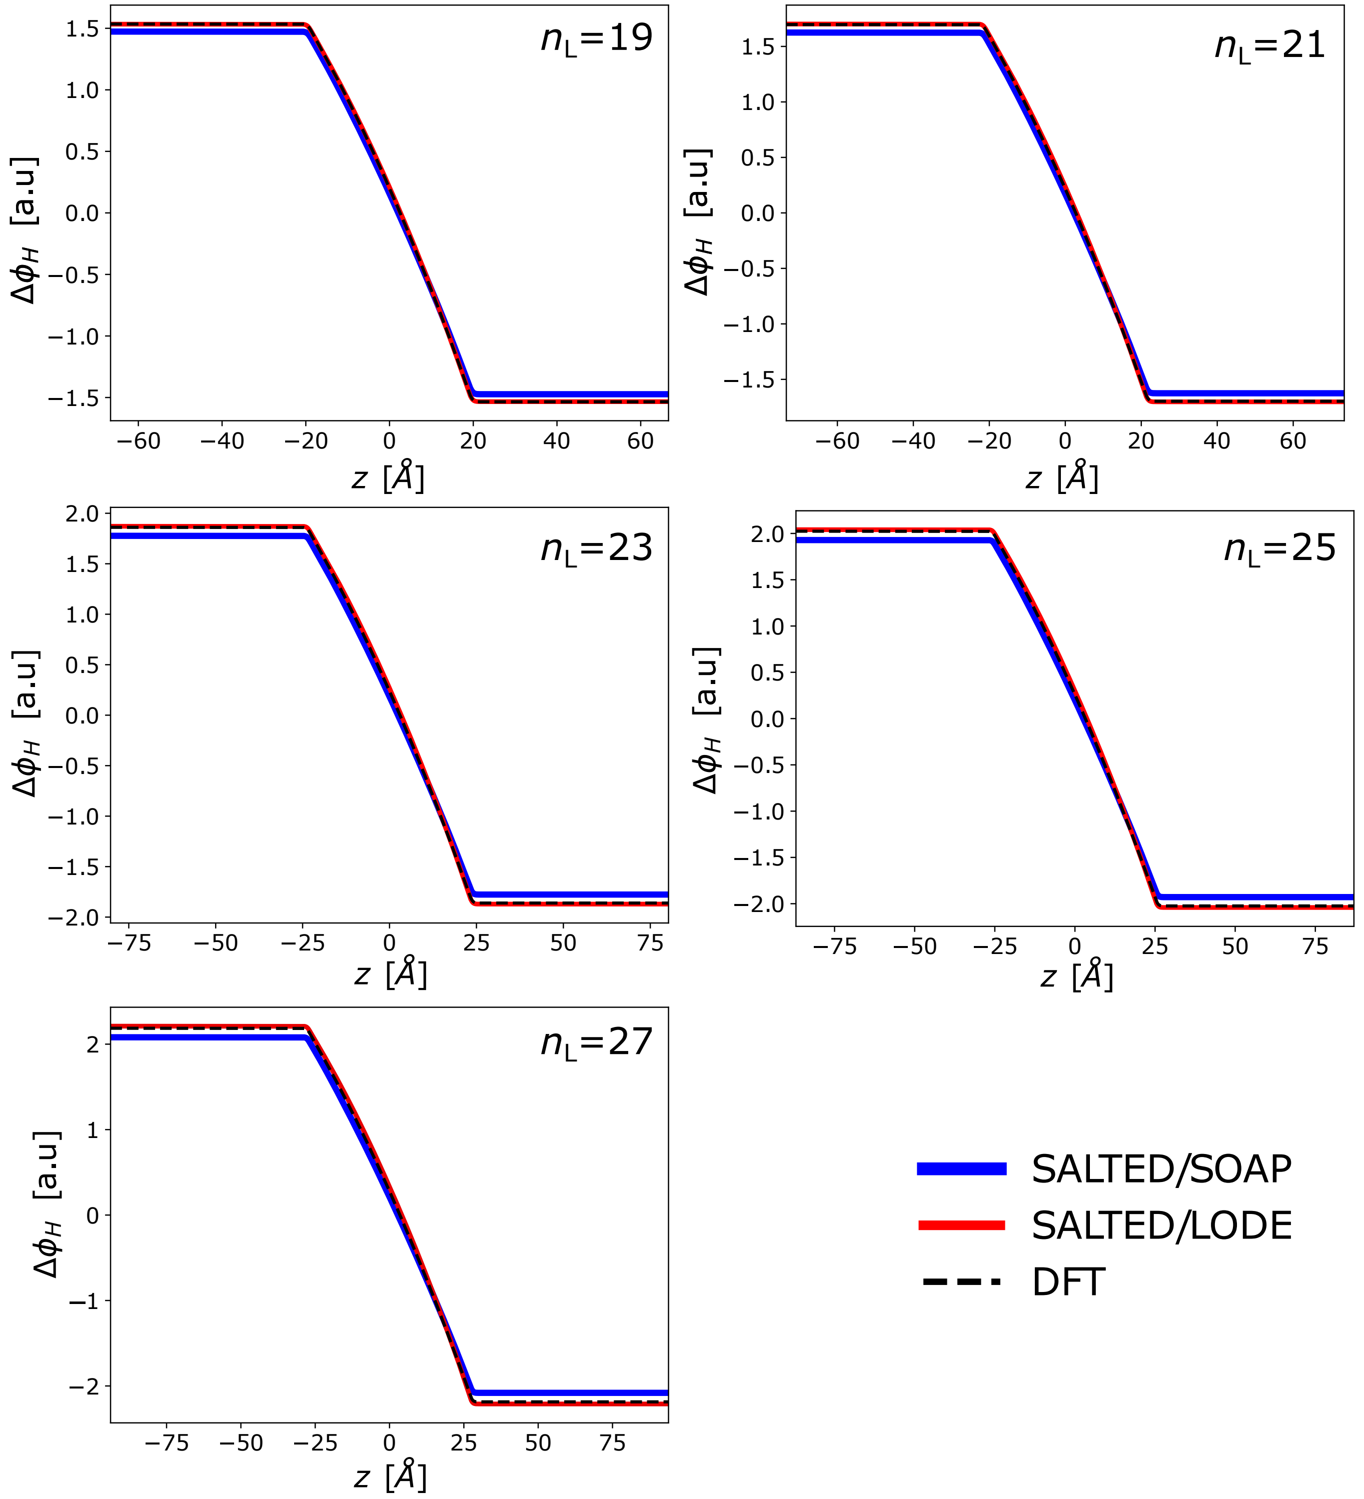


FIG. S2. Longitudinal cut along $z$ of the $Na^+$-induced Hartree potential drop as extrapolated from SALTED/SOAP (blue lines) and SALTED/LODE (red lines) models trained on the QM/MM electron density of Au(100) slabs with $n_{\mathrm{L}}^{max} = 15$ atomic layers, reported for all the test structures considered in this work, i.e., $n_{\mathrm{L}}=\{19, 21, 23, 25, 27\}$. Black dashed line: reference DFT profile.

## IMPORTANCE OF SYMMETRY BREAKING IN FINITE-FIELD PREDICTIONS

We report below a Figure that shows the importance of endowing the structural representation with the symmetry of the applied field along $z$. In particular, we compare predictions of the charge density response for the 27-layers Au(100) electrodes under an applied field obtained through a finite-field SALTED/LODE+E model (as reported in the main text), versus those of a SALTED model that makes use of bare LODE representations. Because of the lack of finite-field information, we observe that a SALTED/LODE model is unable to distinguish structural patterns that are associated with atomic centeres located at the two opposite sides of the metal electrode. As a result, the model is bounded to give perfectly symmetric predictions about the slab center identified by the $z = 0$ plane, and cannot therefore reproduce the asymmetric distribution of electronic charge induced by the applied field. Conversely, mirroring the symmetry of the field in the equivariant structural representations, specifically that associated with ($\lambda = 1$, $\mu = 0$) spherical harmonics, allows us obtain a perfect agreement with respect to DFT.

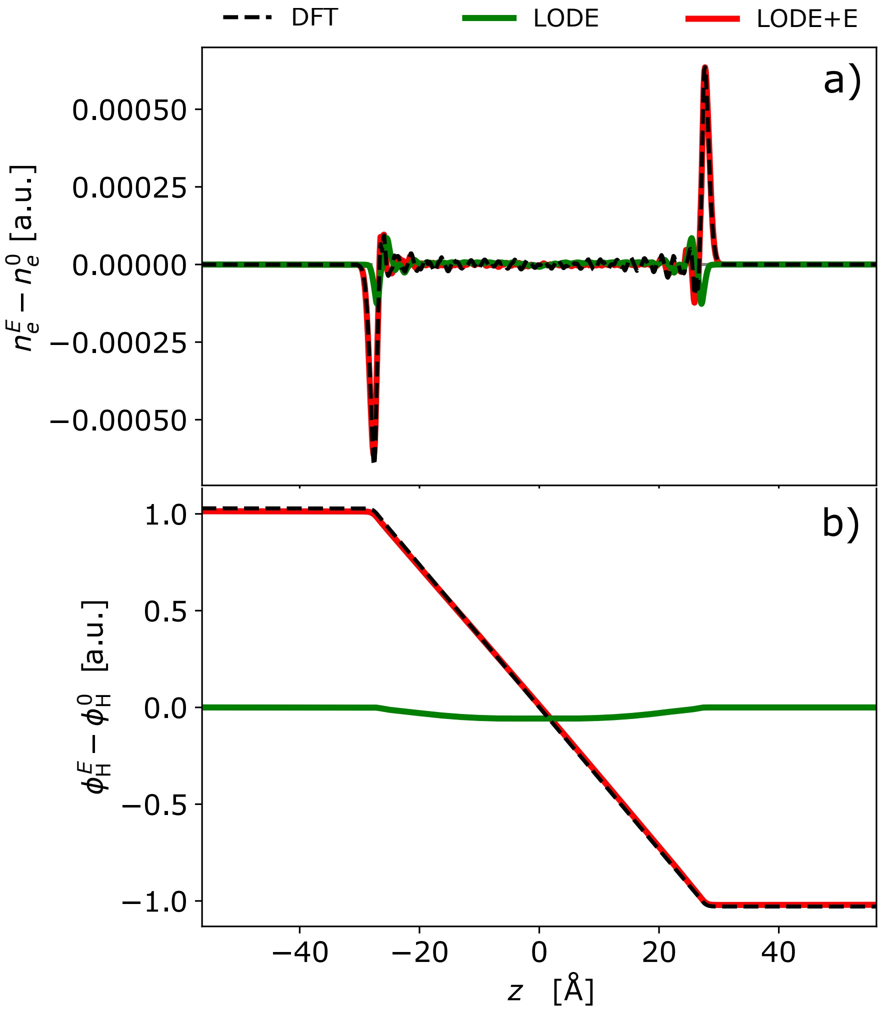


FIG. S3. Predicted electronic response of a 27-layers Au(100) electrode under an applied electric field of $E_z = -1.0$V/Å. a) Charge density response. b) Hartree potential response. Green lines: SALTED/LODE results. Red lines: SALTED/LODE+E results. Black dashed lines: DFT reference.

## VALIDATION OF AU/ELECTROLYTE LEARNING MODEL

We report below learning curves associated with the density-derived prediction of the electronic polarization of the Au(100) electrode for the 400 randomly selected validation structures considered in this work, by also comparing results obtained with different number of sparse atomic environments $M$. Root mean square errors (RMSE) are measured as a fraction of the standard deviation of $p_z$ in the test set. We observe that while the accuracy of the model increases with the number of training structures, increasing the value of $M$ is determinant for lowering the errors of SALTED/LODE predictions below 3% RMSE.

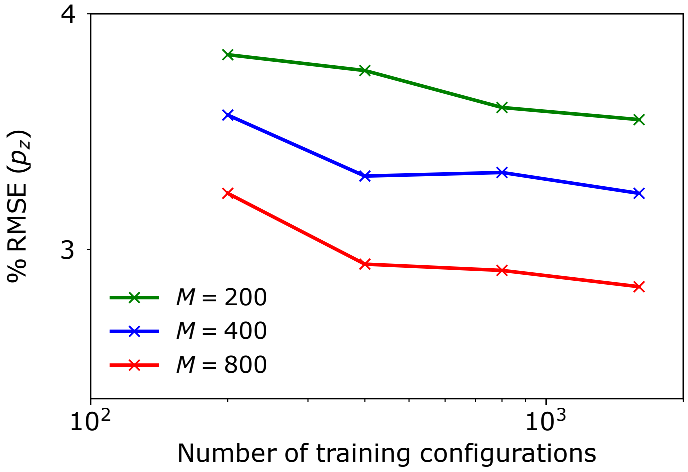


FIG. S4. % Root mean square error of the electrode polarization $p_z$ as predicted from SALTED/LODE models of the charge density response over a test set of 400 electrolyte configurations, reported as a function of the number of training configurations. Learning curves of different color refer to different numbers of sparse atomic environments $M$ used to reduce the dimensionality of the SALTED problem.

For comparison, we also estimate the performance of a SALTED/SOAP model trained with $M = 800$ and $N = 1600$, obtaining a RMSE of 19.5%. We report below a parity plot that compares SALTED/LODE and SALTED/SOAP predictions of $p_z$ against the reference DFT polarization values. Similarly to the Au(100)/Na$^+$ example, SALTED/LODE results are found to outperform those of a local SALTED/SOAP model.

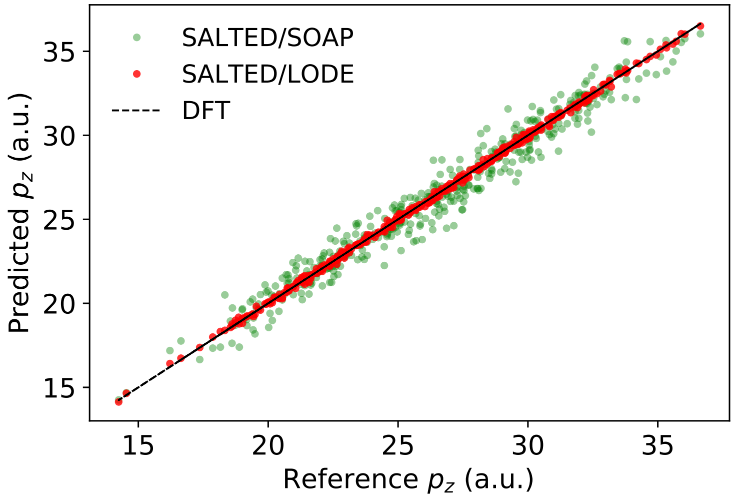


FIG. S5. Comparison of the predicted polarization $p_z$ obtained from SALTED/SOAP (green dots) and SALTED/LODE (red dots) models trained with $M = 800$ and $N = 1600$, reported against the reference DFT values (black dashed line).

Following on the previous discussion, we report below a comparison between SOAP- and LODE-based predictions of the charge-density and Hartree-potential response profiles for a representative Au(100)/electrolyte test configuration

where a local SOAP model fails to accurately reproduce the polarization of the system. The difference between SOAP and LODE is highlighted in the indirect prediction of the Hartree potential difference. In particular, our long-range model is found to accurately reproduce the saw-like behaviour of $\Delta\phi_{\mathrm{H}}$ arising from having performed the reference calculations under 3D period boundary conditions [1].

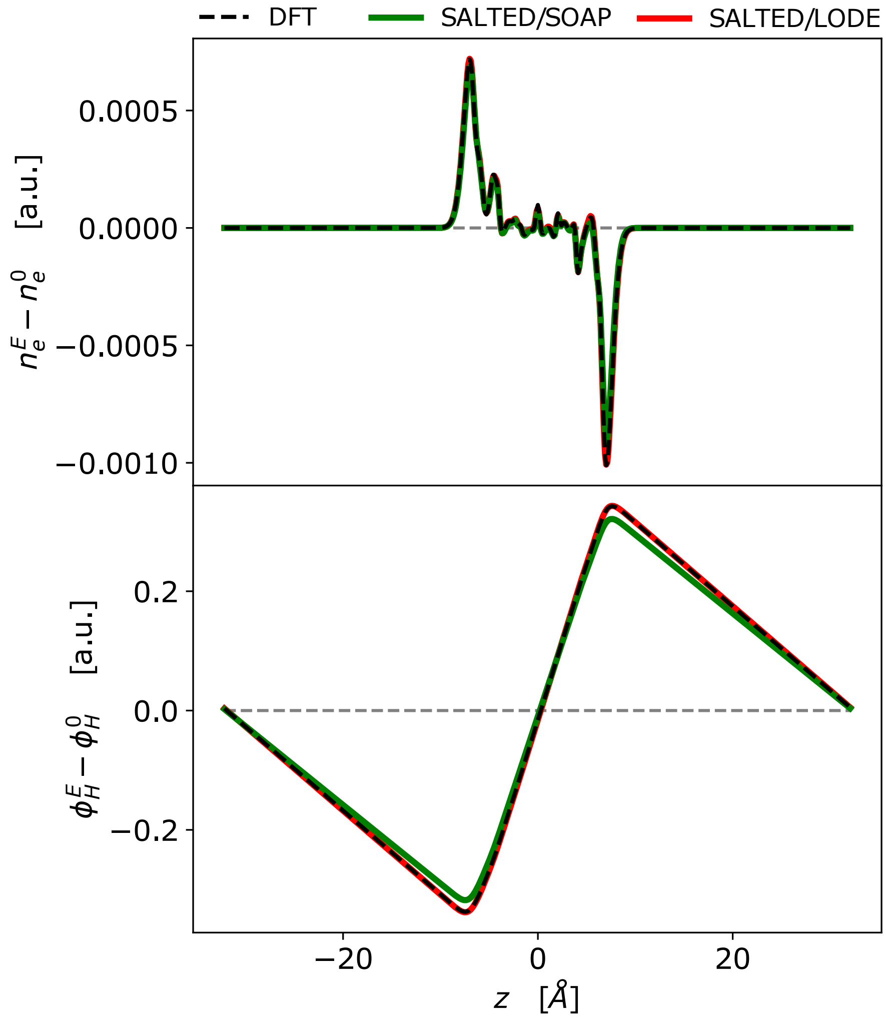


FIG. S6. Predicted electronic response of a representative Au(100)/electrolyte test configuration. a) Charge density response. b) Hartree potential response. Green lines: SALTED/SOAP. Red lines: SALTED/LODE. Black dashed lines: DFT.

## CALCULATION OF THE DIFFERENTIAL CAPACITANCE FOR THE AU/ELECTROLYTE INTERFACE

The calculation of the differential capacitance $C_{\mathrm{diff}}$ follows the result of Ref. [22]. In particular, we refer to the electrical double-layer (EDL) contribution to $C_{\mathrm{diff}}$, which can be computed from the electrolyte-induced fluctuations of the electrode surface charge. In the case of the 3D-periodic Au/electrolyte example shown in this work, this implies that we can rely on the formula

$$C_{\mathrm{diff}}^{\mathrm{EDL}} = \beta \left\langle (Q - \langle Q \rangle)^2 \right\rangle , \tag{S18}$$

where $Q$ represents the accumulation/depletion of opposite electronic charge at the two sides of the metal electrode. Computing $Q$ from SALTED/LODE predictions of the charge density response implies taking either the right or left integral $\Delta n_e$ from the middle of the slab to the classical electrolyte region. This can be computed analytically from the isotropic ($\lambda = 0$, $\mu = 0$) density coefficients of the atoms that belong to one of the two sides of the metallic slab.

For instance, setting the central metal layer at $z = 0$ we can write:

$$Q_{\rm right} = -\sqrt{4\pi} \sum_{i \in z>0} c_i^{n00} \sum_n \int_0^\infty dr\, r^2\, R_n^0(r)\,. \tag{S19}$$

We report below a comparison between the MetalWalls and SALTED/LODE right charge integral, $Q_{\rm right}$, computed over the 5500 uncorrelated frames used to estimate the differential capacitance of the system.

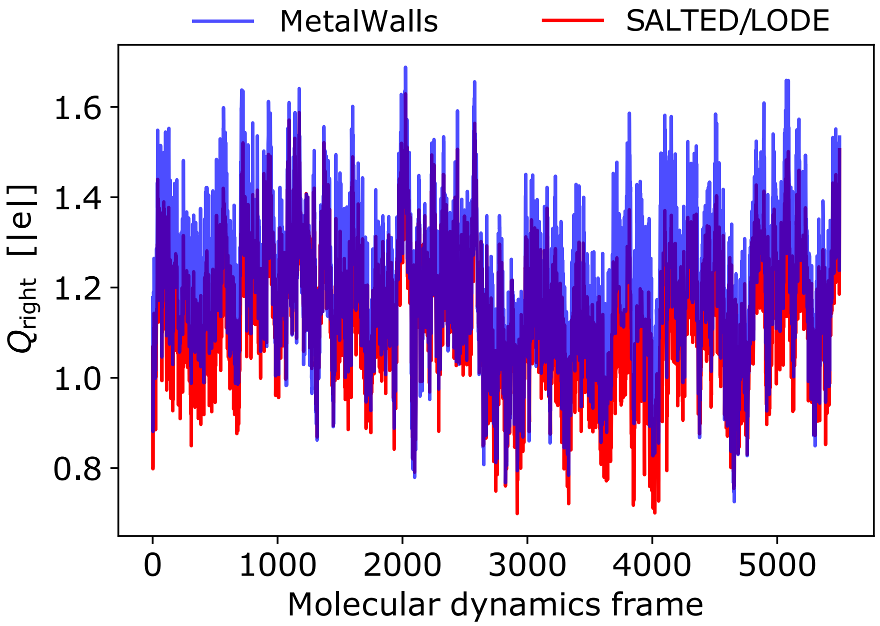


FIG. S7. Predicted integrated charge variations on the right hand side of the Au(100) electrode induced by the electrolyte distribution over a molecular dynamics trajectory. Blue line: MetalWalls results. Red line: SALTED/LODE results.

* andrea.grisafi@ens.psl.eu

[S1] T. Dufils, G. Jeanmairet, B. Rotenberg, M. Sprik, and M. Salanne, Phys. Rev. Lett. **123**, 195501 (2019).
[S2] A. Marin-Laflèche, M. Haefele, L. Scalfi, A. Coretti, T. Dufils, G. Jeanmairet, S. K. Reed, A. Serva, R. Berthin, C. Bacon, S. Bonella, B. Rotenberg, P. A. Madden, and M. Salanne, Journal of Open Source Software **5**, 2373 (2020).
[S3] S. Nosé, J. Chem. Phys. **81**, 511 (1984).
[S4] J. L. F. Abascal and C. Vega, The Journal of Chemical Physics **123**, 234505 (2005).
[S5] T. D. Kühne, M. Iannuzzi, M. Del Ben, V. V. Rybkin, P. Seewald, F. Stein, T. Laino, R. Z. Khaliullin, O. Schütt, F. Schiffmann, D. Golze, J. Wilhelm, S. Chulkov, M. H. Bani-Hashemian, V. Weber, U. Borštnik, M. Taillefumier, A. S. Jakobovits, A. Lazzaro, H. Pabst, T. Müller, R. Schade, M. Guidon, S. Andermatt, N. Holmberg, G. K. Schenter, A. Hehn, A. Bussy, F. Belleflamme, G. Tabacchi, A. Glöß, M. Lass, I. Bethune, C. J. Mundy, C. Plessl, M. Watkins, J. VandeVondele, M. Krack, and J. Hutter, The Journal of Chemical Physics **152**, 194103 (2020).
[S6] S. Goedecker, M. Teter, and J. Hutter, Physical Review B **54**, 1703 (1996).
[S7] G. J. Martyna and M. E. Tuckerman, The Journal of Chemical Physics **110**, 2810 (1999).
[S8] P. Mináry, M. E. Tuckerman, K. A. Pihakari, and G. J. Martyna, The Journal of Chemical Physics **116**, 5351 (2002).
[S9] T. Laino, F. Mohamed, A. Laio, and M. Parrinello, Journal of Chemical Theory and Computation **2**, 1370 (2006).
[S10] A. Bussy, O. Schütt, and J. Hutter, The Journal of Chemical Physics **158**, 164109 (2023).
[S11] G. L. Stoychev, A. A. Auer, and F. Neese, Journal of Chemical Theory and Computation **13**, 554 (2017).
[S12] A. Grisafi, J. Nigam, and M. Ceriotti, Chem. Sci. **12**, 2078 (2021).
[S13] M. J. Willatt, F. Musil, and M. Ceriotti, J. Chem. Phys. **150**, 154110 (2019).
[S14] A. Grisafi, D. M. Wilkins, M. J. Willatt, and M. Ceriotti, in *Machine Learning in Chemistry*, Vol. 1326, edited by E. O. Pyzer-Knapp and T. Laino (American Chemical Society, Washington, DC, 2019) pp. 1–21.
[S15] A. Grisafi and M. Ceriotti, J. Chem. Phys. **151**, 204105 (2019).
[S16] F. Musil, A. Grisafi, A. P. Bartók, C. Ortner, G. Csányi, and M. Ceriotti, Chemical Reviews **121**, 9759 (2021).
[S17] A. Grisafi, A. M. Lewis, M. Rossi, and M. Ceriotti, Journal of Chemical Theory and Computation **19**, 4451 (2023).
[S18] G. Imbalzano, A. Anelli, D. Giofré, S. Klees, J. Behler, and M. Ceriotti, J. Chem. Phys. **148**, 241730 (2018).

[S19] A. Grisafi, D. M. Wilkins, G. Csányi, and M. Ceriotti, Phys. Rev. Lett. **120**, 036002 (2018).
[S20] A. Grisafi, A. Fabrizio, B. Meyer, D. M. Wilkins, C. Corminboeuf, and M. Ceriotti, ACS Cent. Sci. **5**, 57 (2019).
[S21] G. Fraux, P. Loche, S. Kliavinek, K. K. Huguenin-Dumittan, D. Tisi, and A. Goscinski, "rascaline," .
[S22] L. Scalfi, D. T. Limmer, A. Coretti, S. Bonella, P. A. Madden, M. Salanne, and B. Rotenberg, Phys. Chem. Chem. Phys. **22**, 10480 (2020).
